# Supplementary material for: SC4D: Sparse-Controlled Video-to-4D Generation and Motion Transfer
Source: arXiv:2404.03736 source file (2024-08-14)
Supplement: Supplementary file 1 [file 7_Supp.tex]

\section{More Implementation Details}
\label{supp_details}

\noindent\textbf{Video-to-4D Generation.}
In the coarse stage, we perform densification and pruning every 100 iterations in the first 1,000 iterations with a gradient threshold of 0.01 and opacity threshold of 0.01. Then in the remaining 500 iterations of the coarse stage, we only perform pruning with an interval of 100 iterations. The sampled timestep in the coarse stage is between [600, 800] in a linear decrease manner to ensure shape plausibility. In the fine stage, we only perform pruning every 1,000 iterations instead of densification. And the sampled timestep decreases from 800 to 200 for detailed texture. In both stages, the learning rates for Gaussians' rotation, opacity, scaling, and color equal 0.005, 0.05, 0.05, and 0.01, respectively. The learning rate for control points' control radius is set to 0.005. The Gaussians' position learning rate in the coarse stage decreases linearly from 0.01 to 0.0002 and remains 0.0002 in the fine stage. The learning rate for deformation MLP parameters equals 0.0002 in the coarse stage, and then gradually decreases to 2e$^{-6}$ in the fine stage.

\noindent\textbf{Motion Transfer Application.}
During the first 1,000 training iterations, the sampled timestep undergoes a linear decrease from 980 to 20. In the following 1,000 iterations, the timestep reduces from 200 to 20. The dense Gaussians' position learning rate is set to 0.0002, while other trainable Gaussian parameters are consistent with those used in in the video-to-4D pipeline. 

\noindent\textbf{Temporal Error.}
As described in the main paper, we utilize Temporal Error as a measurement for temporal consistency and motion fidelity. To do so, we adopt the RAFT~\cite{raft} model pretrained on KITTI2015~\cite{kitti} dataset provided by MMFlow~\cite{mmflow} as the optical flow estimator. Given a video of the generated dynamic object projected from the reference view and the corresponding reference video, we first feed the initial two frames of the reference video into the optical flow estimator to obtain the predicted forward optical flow. Subsequently, we use the predicted optical flow to warp the first frame of the synthesized video. The warped frame is then compared against the second frame of the synthesized video by computing the L2 distance between them, which serves as the final result. We employ this procedure to calculate the corresponding outcomes for all adjacent frames of the video, and the average of these results is used as the final Temp Error (Temp).

\section{Details of User Study}
\label{supp_user}
In the user study questionnaire, we choose 10 videos with large motion from the Consistent4D~\cite{con4d} dataset, which are: \textit{triceratops}, \textit{guppie}, \textit{robot}, \textit{rabbit}, \textit{patrick}, \textit{jack}, \textit{ironman}, \textit{elephant}, \textit{egret}, \textit{aurorus}, respectively. Utilizing the above videos as references, we train the compared methods to obtain the dynamic objects. We then project each object from a reference viewpoint and a random viewpoint, yielding $2\times 3=6$ options for each question. We ask each participant to choose one option from the reference viewpoint and one from the novel viewpoint according to the reference view alignment, spatio-temporal consistency, and motion fidelity. The options for each question are randomly shuffled to avoid biases. 
% We attach the questionnaire and all the involved videos in the $User~Study$ folder. 

\section{More Quantitative Comparisons}
\label{supp_quant}
Following Consistent4D~\cite{con4d}, we use the same testset and evaluation script to measure the performance of the compared methods. The results are shown in Tab.~\ref{tab:supp_quant}. Different from the evaluation in our main paper, the testset in Consistent4D contains four novel view ground truth renderings, apart from the reference video frames. The metrics are calculated between projections of the generated dynamic object and the corresponding rendering under the same viewpoint. We argue that this evaluation approach is less reasonable since the novel view information of the compared methods originates from Zero123~\cite{zero123}, and the prior knowledge in Zero123 might not align with the real data. Moreover, the values in Tab.~\ref{tab:supp_quant} are too close, which misaligns with the qualitative results and user study, further revealing the necessity of the evaluations in our main paper. Additionally, we observe that the test samples from the consistent4D dataset exhibit relatively minor movements. In order to better assess and compare the robustness of various methods in learning motion, we have supplemented with some examples that demonstrate larger movements. 
% We include all the detailed quantitative evaluation in the $Quantitative~Evaluations$ folder.

\begin{table}[ht]
\centering
\caption{Quantitative evaluations according to Consistent4D~\cite{con4d}.}
\vspace{-.1in}
% \resizebox{0.9\linewidth}{!}{
\begin{tabular}{lcc}
\toprule[1pt] 
    Method & CLIP~$\uparrow$ & LPIPS~$\downarrow$   \\
    \midrule 
    Consistent4D~\cite{con4d} & 0.91 & \textbf{0.14}    \\
    4DGen~\cite{4dgen} & 0.91 & \textbf{0.14}    \\
    SC4D(Ours) & \textbf{0.92} & \textbf{0.14}   \\
\bottomrule[1pt] 
\end{tabular} 
% }
\vspace{-.2in}
\label{tab:supp_quant}
\end{table}

\section{More Ablation Studies}
\label{supp_abl}

\subsection{Number of Control Points}
We conduct experiments to verify the influences on the number of control points (denoted as $M$). We experiment on the example of \textit{frog} here due to its complex motion. The results are shown in Tab.~\ref{tab:num_cpts}. As we can see, as $M$ grows larger, the reference view alignment (PSNR, SSIM, LPIPS) and multi-view consistency (CLIP) of the generated dynamic object improve, which indicates that with more control points, the details of each view can be better restored. However, the temporal consistency degrades simultaneously, which reveals the degeneration of local rigidity when the number of control points is more significant. As a compromise, we choose $M=512$ as our default setting.

\begin{table}[ht]
\centering
\caption{Ablation study on the number of control points (denoted as \textit{M}).}
\vspace{-.1in}
% \resizebox{0.9\linewidth}{!}{
\begin{tabular}{cccccc}
\toprule[1pt] 
    \textit{M} & PSNR~$\uparrow$ & SSIM~$\uparrow$ & LPIPS~$\downarrow$ & CLIP~$\uparrow$ & Temp~$\downarrow$   \\
    \midrule 
    128 & 26.46 & 0.934 & 0.084 & 0.890 & \textbf{0.0175}   \\
    256 & 26.75 & 0.936 & 0.080 & 0.890 & 0.0176   \\
    512 & 27.00 & 0.936 & \textbf{0.078} & \textbf{0.893} & 0.0178   \\
    1024 & \textbf{27.30} & \textbf{0.938} & 0.079 & \textbf{0.893} & 0.0180   \\
\bottomrule[1pt] 
\end{tabular} 
% }
%\vspace{-.1in}
\label{tab:num_cpts}
\end{table}

\subsection{Comparison between GA Loss and the Chamfer Loss}
As illustrated in Fig.~\ref{fig:abl_ga}, when utilizing the Chamfer loss to prevent the shape degeneration issue, the control points tend to cluster around certain points especially when the loss weight grows larger, resulting in an uneven distribution. In comparison, our proposed GA loss can prevent shape degeneration without hurting the overall distribution of control points.

\begin{figure}[ht]
\begin{center}
\includegraphics[width=0.98\textwidth]{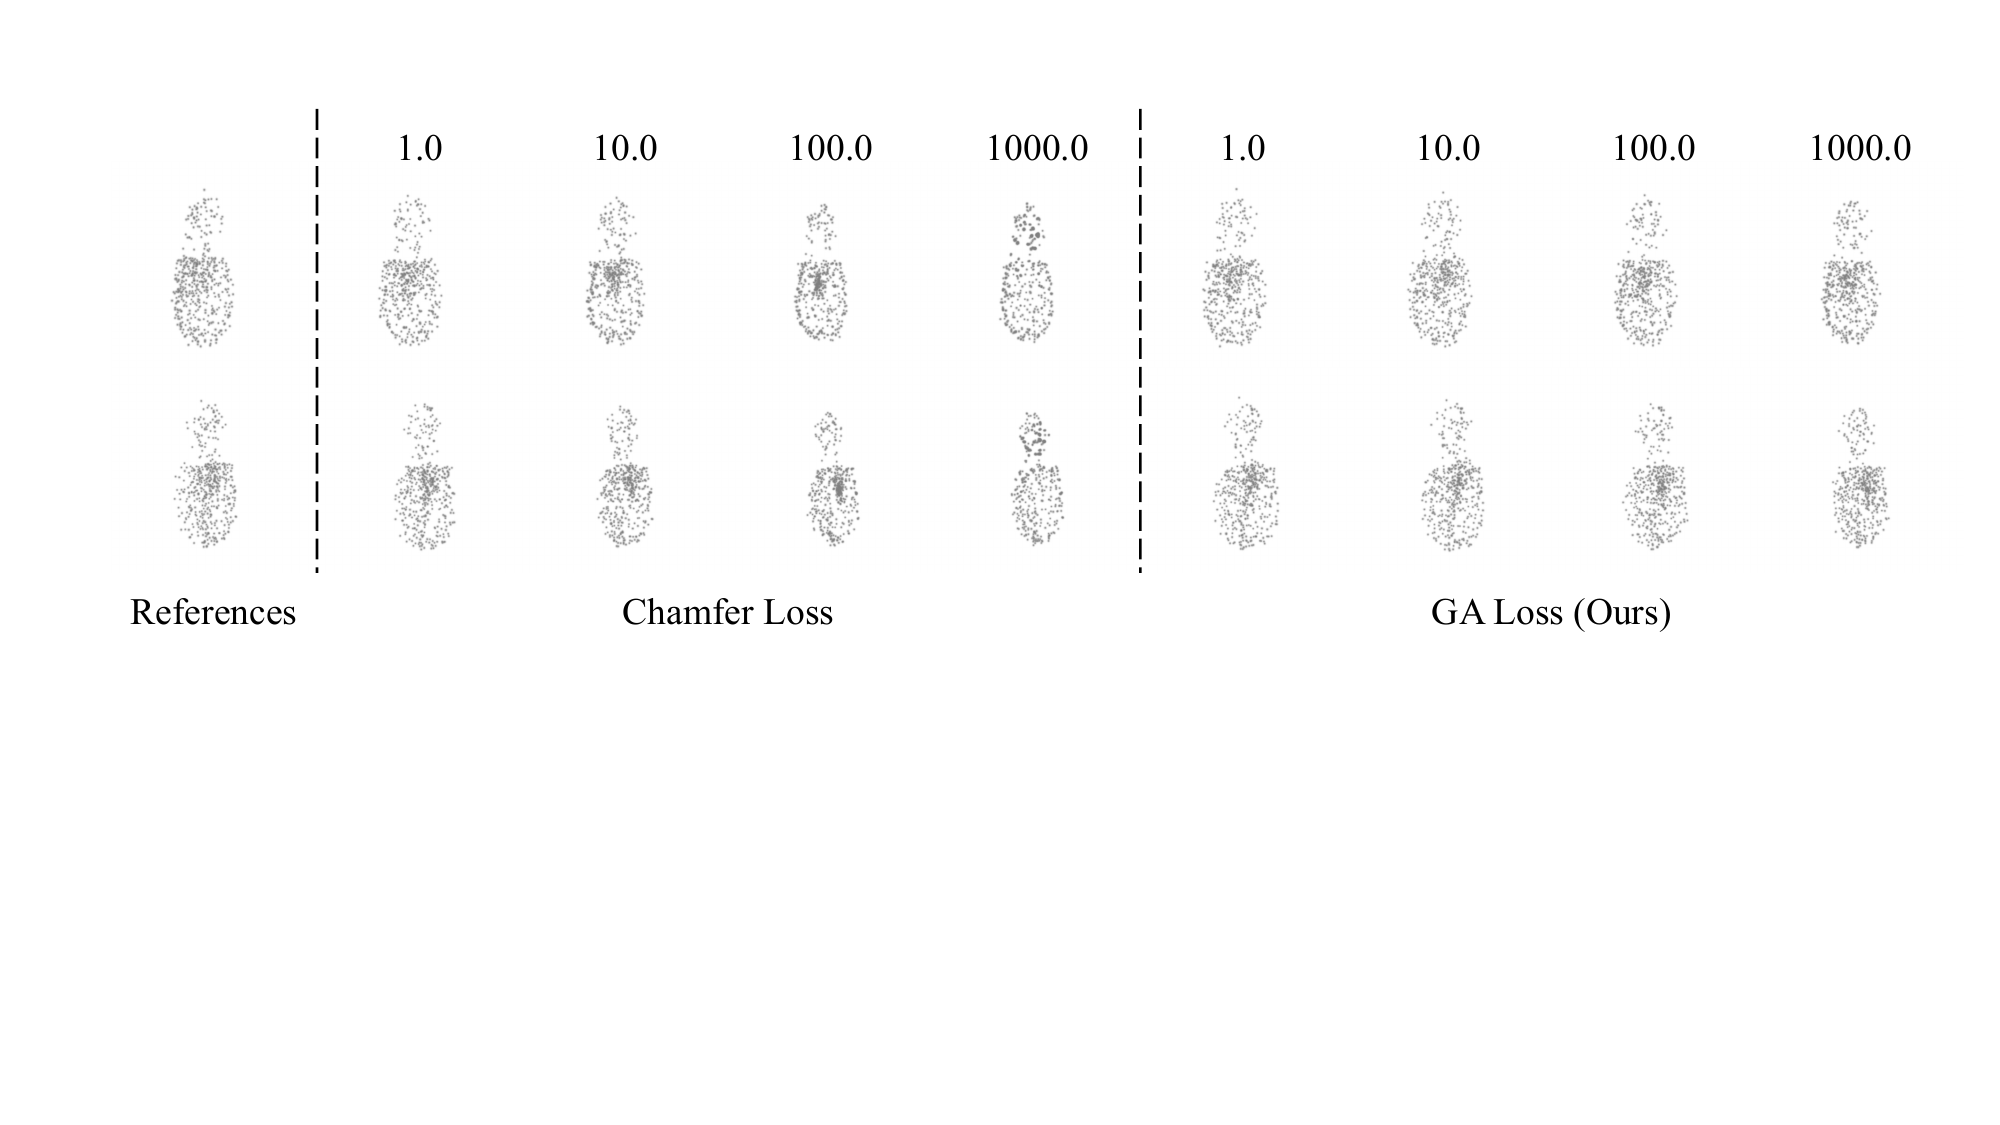}
\end{center}
\vspace{-.2in}
\caption{Qualitative comparison on the effect of the proposed GA loss against the Chamfer loss. We attach the loss weight above each instance. The reference control points are the ones in the coarse stage from two different viewpoints.}
\label{fig:abl_ga}
\end{figure}

\subsection{Comparison between AG Initialization and Direct Initialization}
In the main paper, we compare the proposed AG initialization with $Ori~init$, which represents initializing dense Gaussians within a sphere in the canonical space as in the coarse stage. In fact, there is another naive initialization approach that directly utilizes the control Gaussians as initialization of the fine stage, which we call $Direct~init$. As shown in Fig.~\ref{fig:abl_init}, $Direct~init$ also leads to shape degeneration issue, illustrated by the over-thickness of the deforming toy rabbit.

\begin{figure}[!t]
\begin{center}
\includegraphics[width=0.60\textwidth]{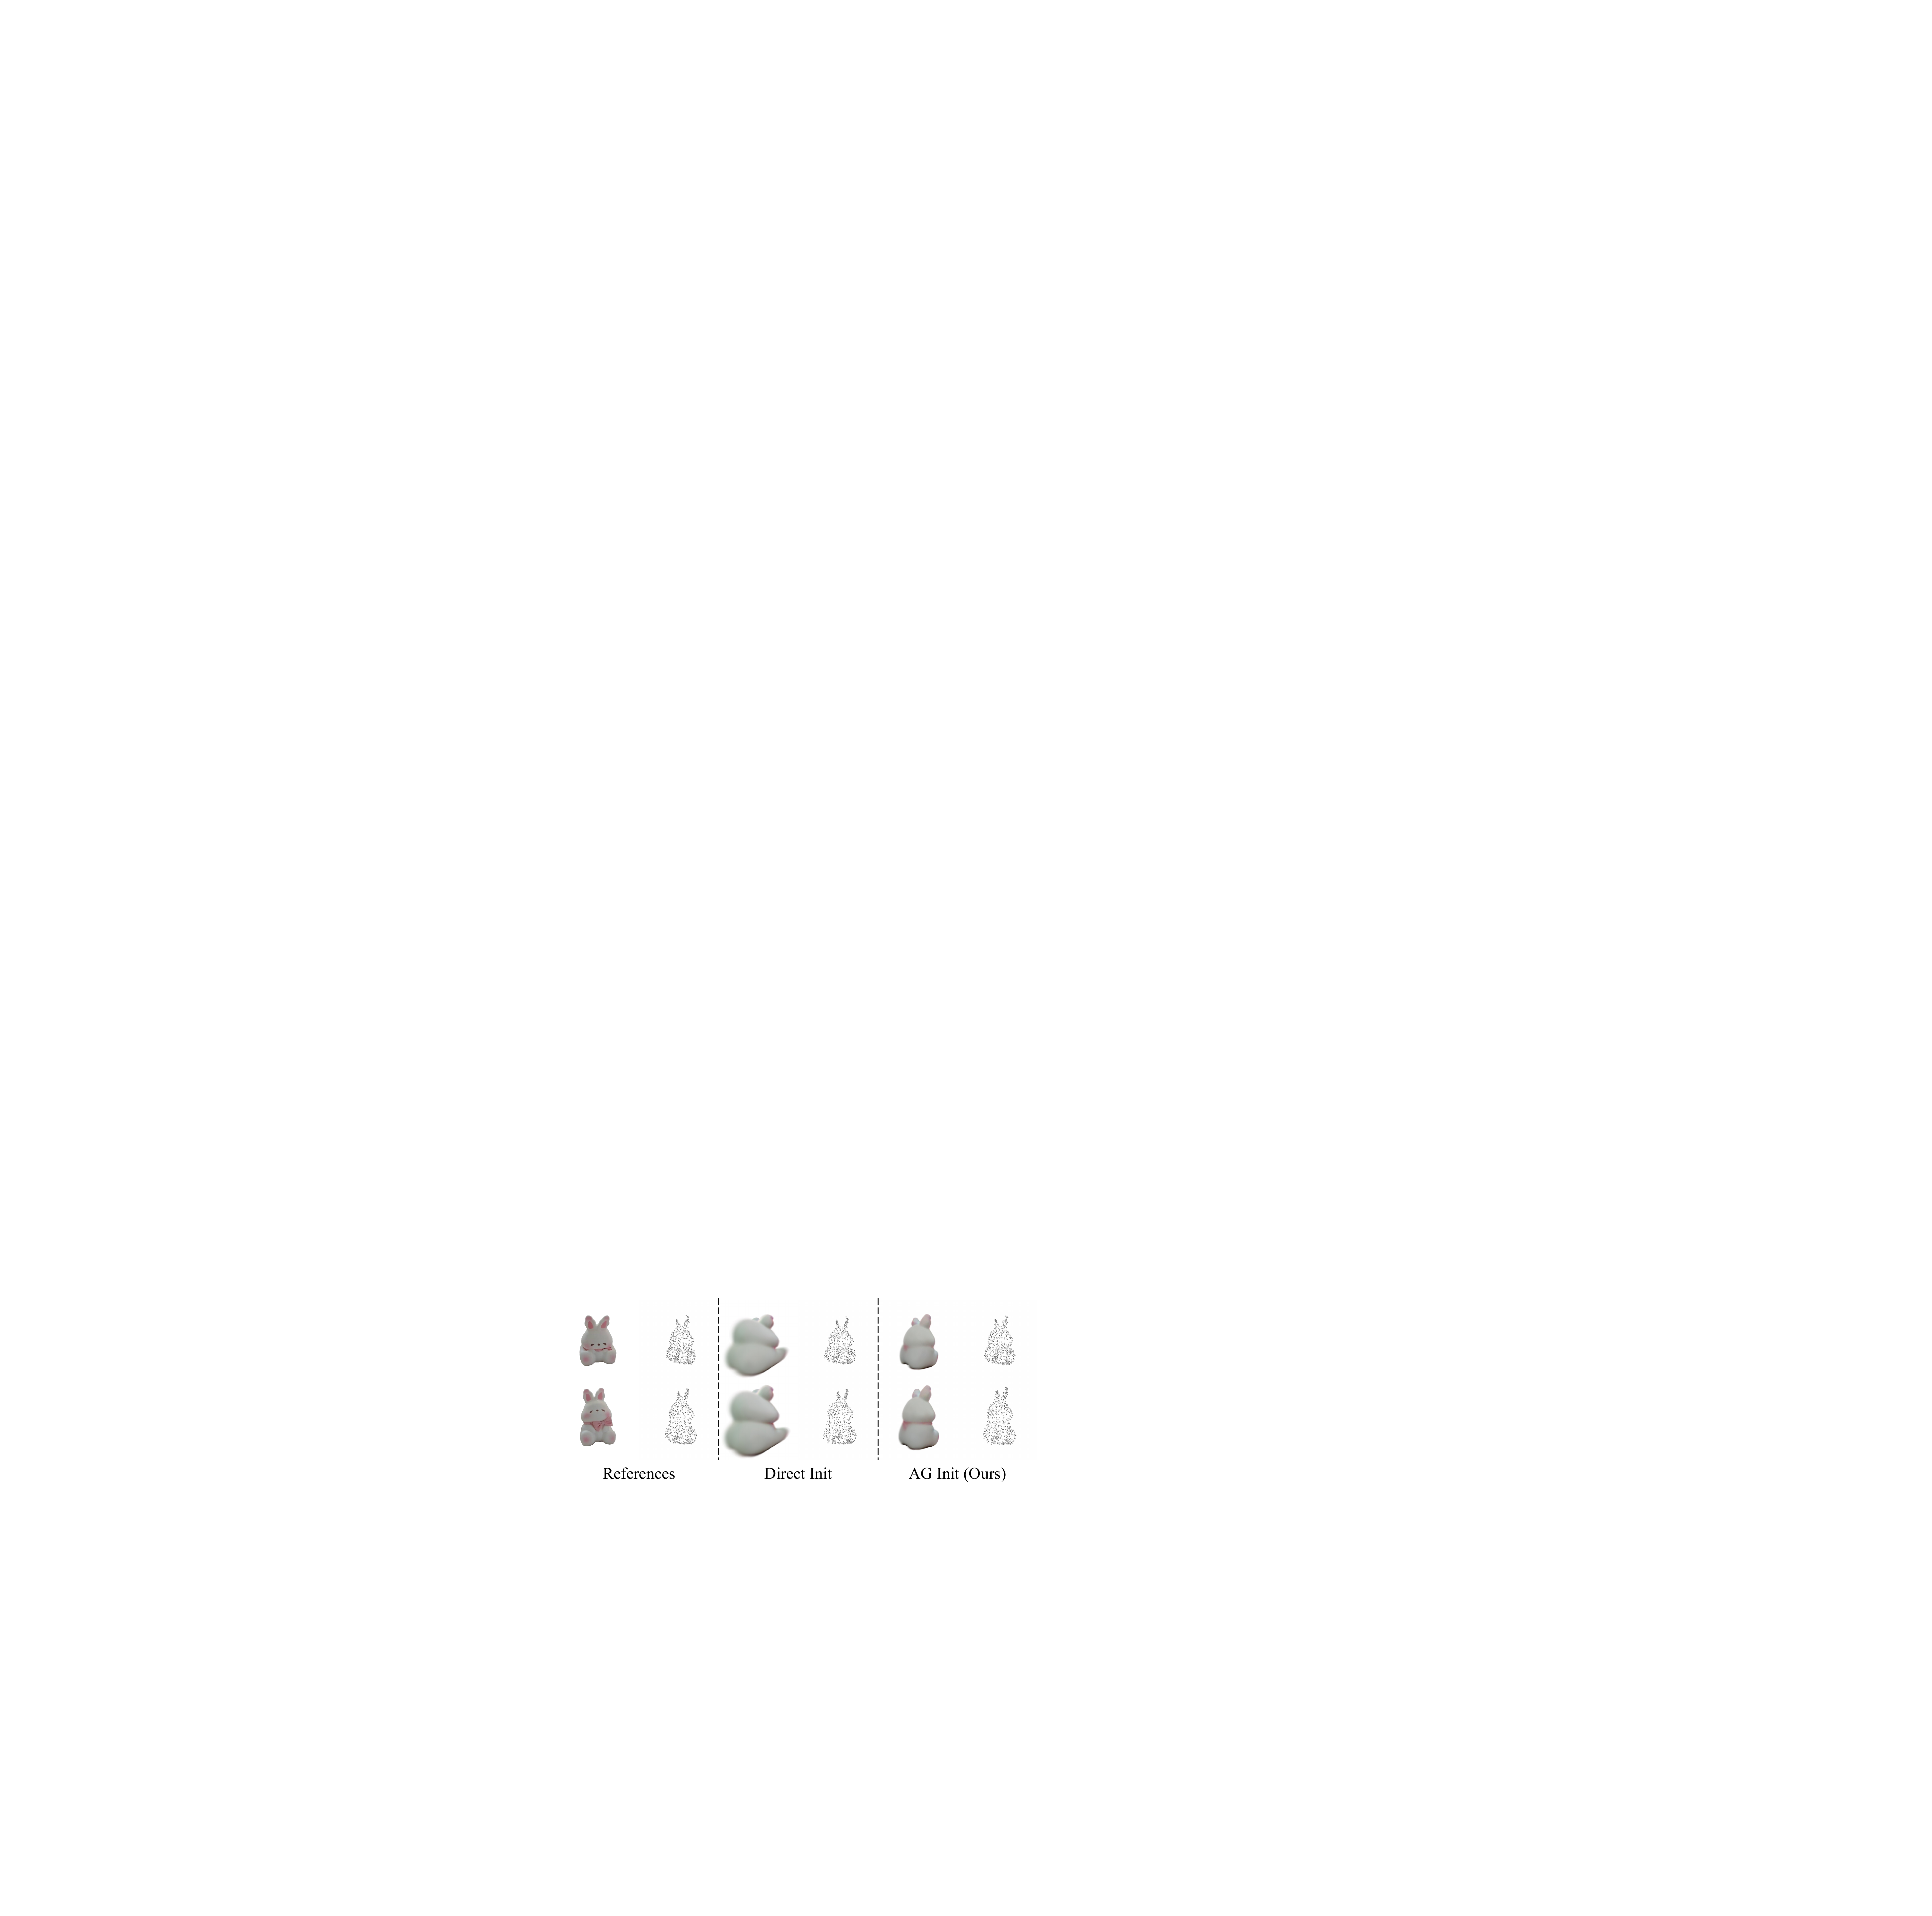}
\end{center}
\vspace{-.2in}
\caption{Comparison between the proposed AG initialization and the Direct initialization. The latter represents directly utilizing the control Gaussians in the coarse stage as the initialization of the fine stage.}
\label{fig:abl_init}
\end{figure}

%\subsection{Number of Densification}

\section{More Qualitative Comparisons}
\label{supp_qua}
We show more qualitative comparisons in Fig.~\ref{fig:supp_qua}. The results illustrate the effectiveness and robustness of SC4D.

\begin{figure}[!t]
\begin{center}
\includegraphics[width=0.98\textwidth]{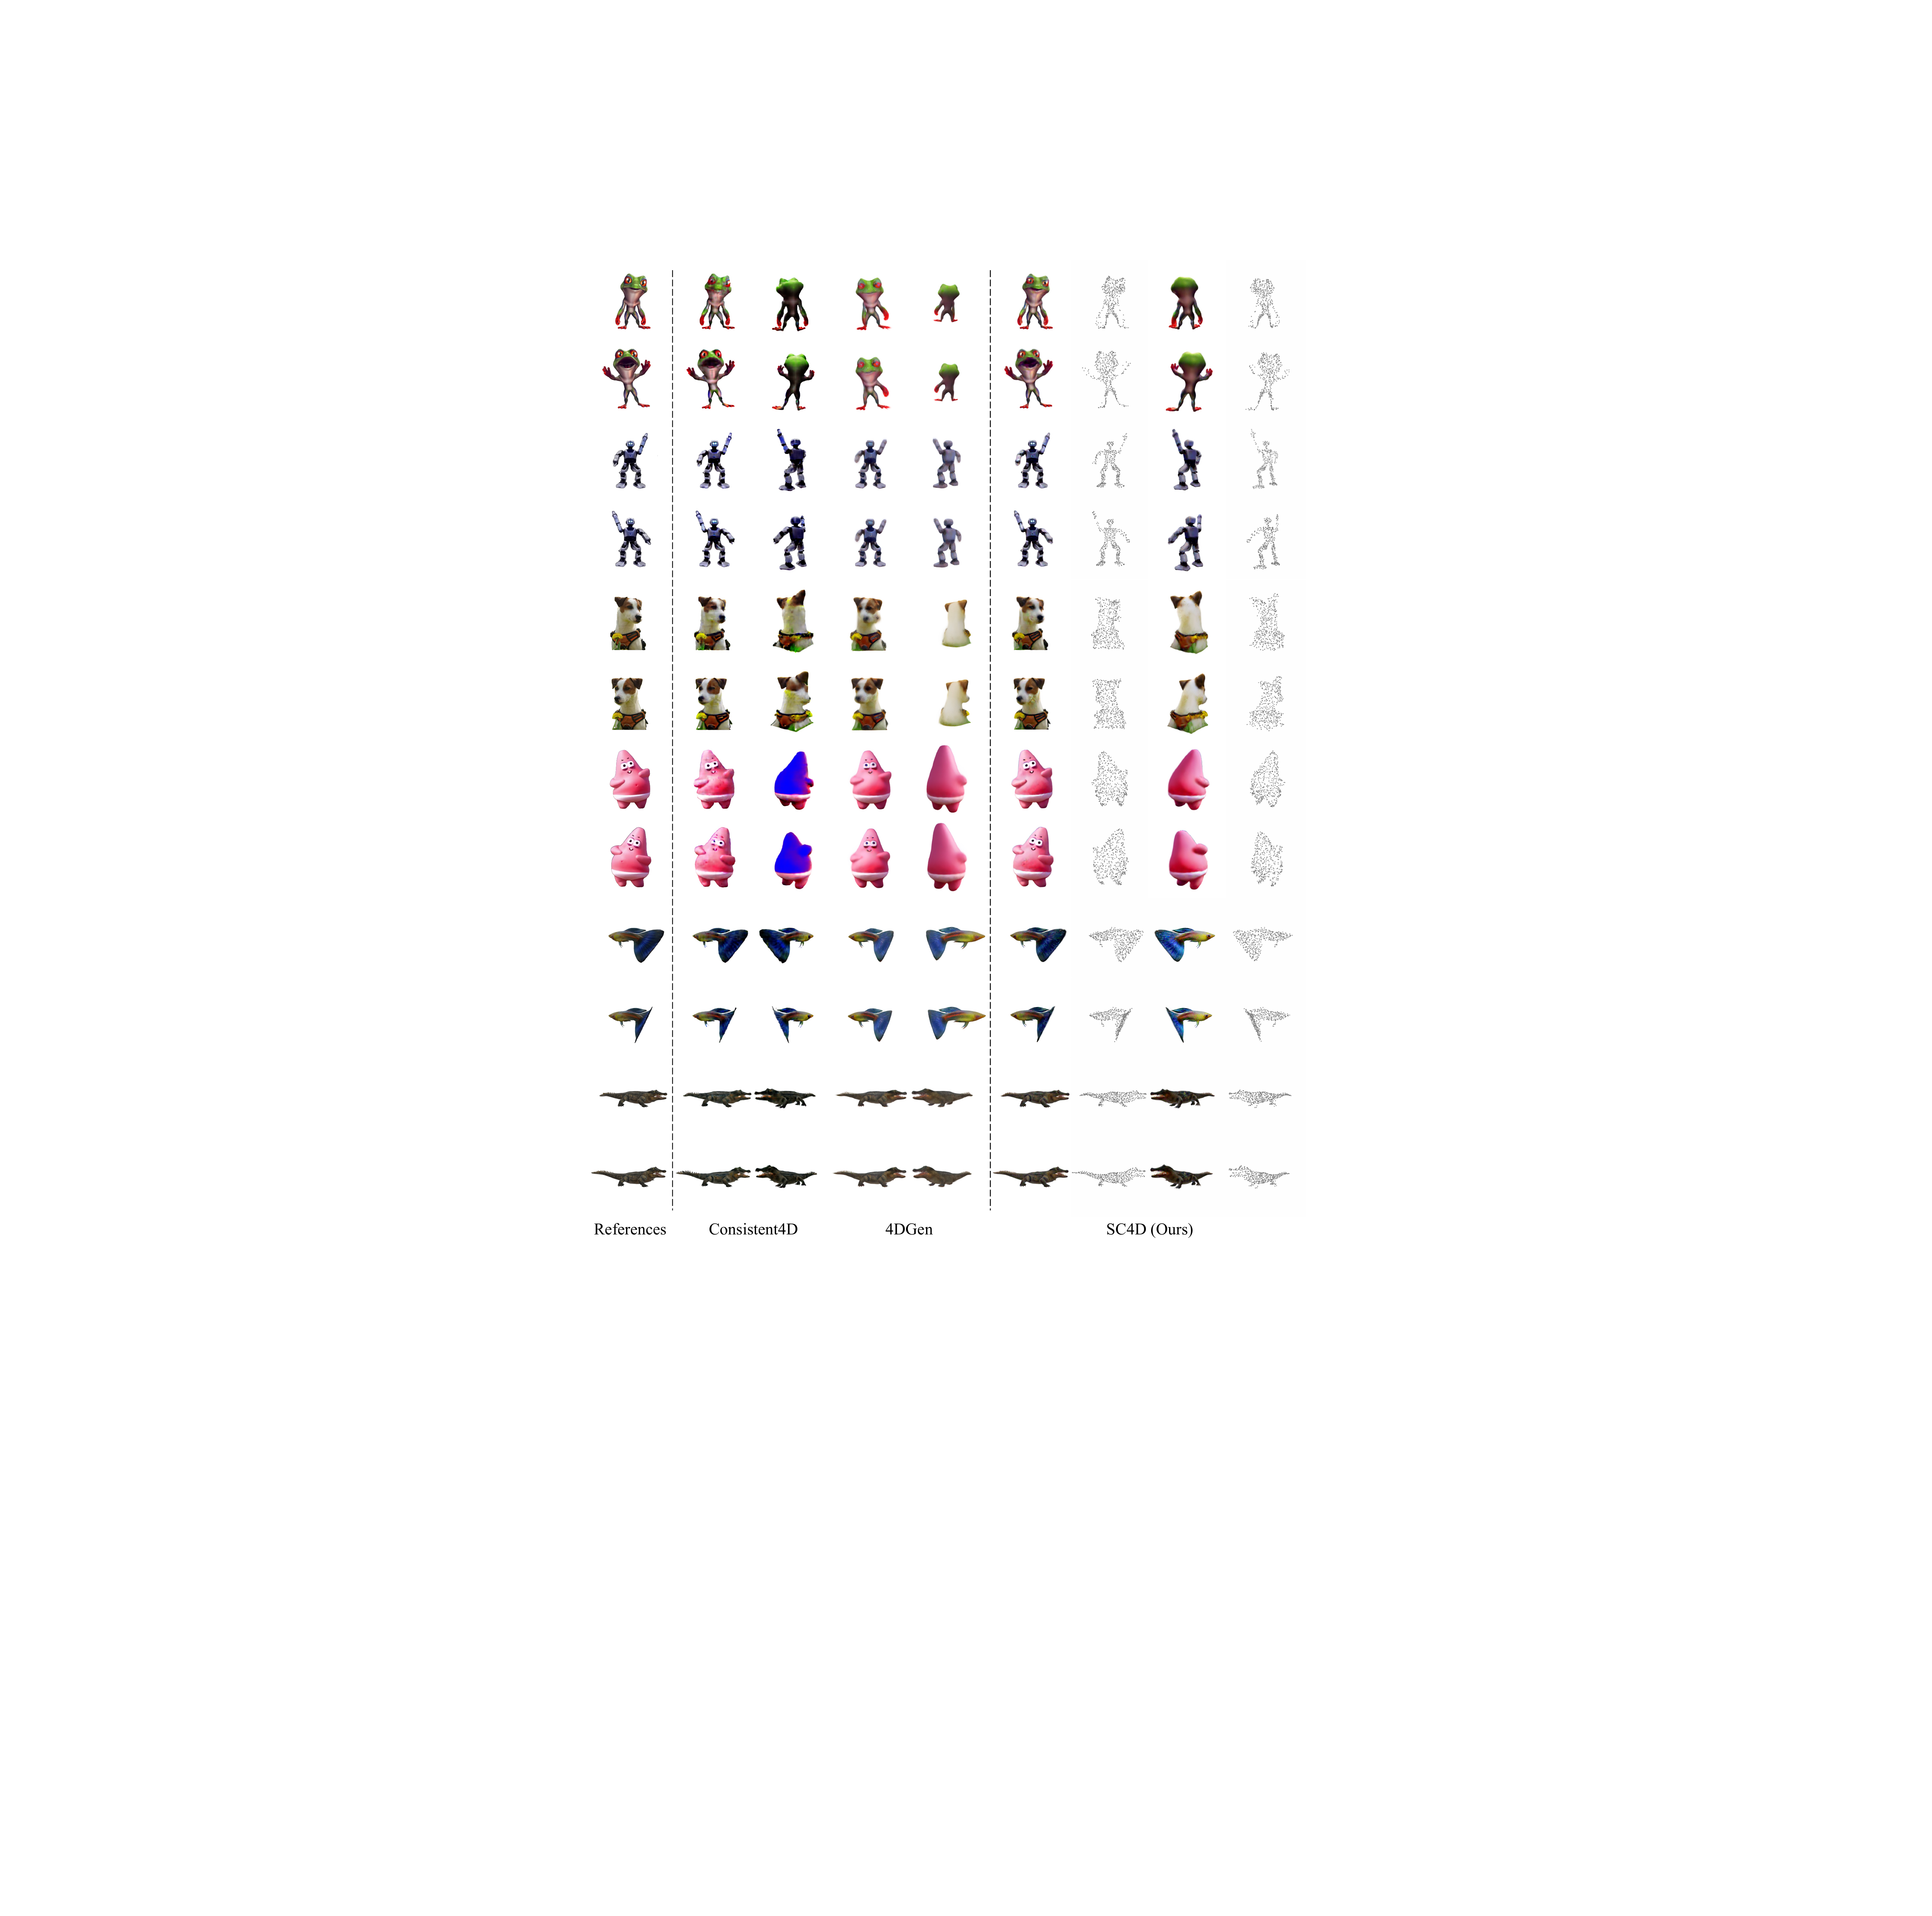}
\end{center}
\vspace{-.2in}
\caption{Additional qualitative comparisons. (Best viewed when zoomed in.)}
\label{fig:supp_qua}
\end{figure}

\section{More Application Examples}
\label{supp_app}
We show more application examples in Fig.~\ref{fig:supp_app}. These examples demonstrate the flexibility of the proposed motion transfer application. 
% We attach the motion application results and corresponding reference videos in the folder: $Application$ $Examples$.

\begin{figure}[!t]
\begin{center}
\includegraphics[width=0.98\textwidth]{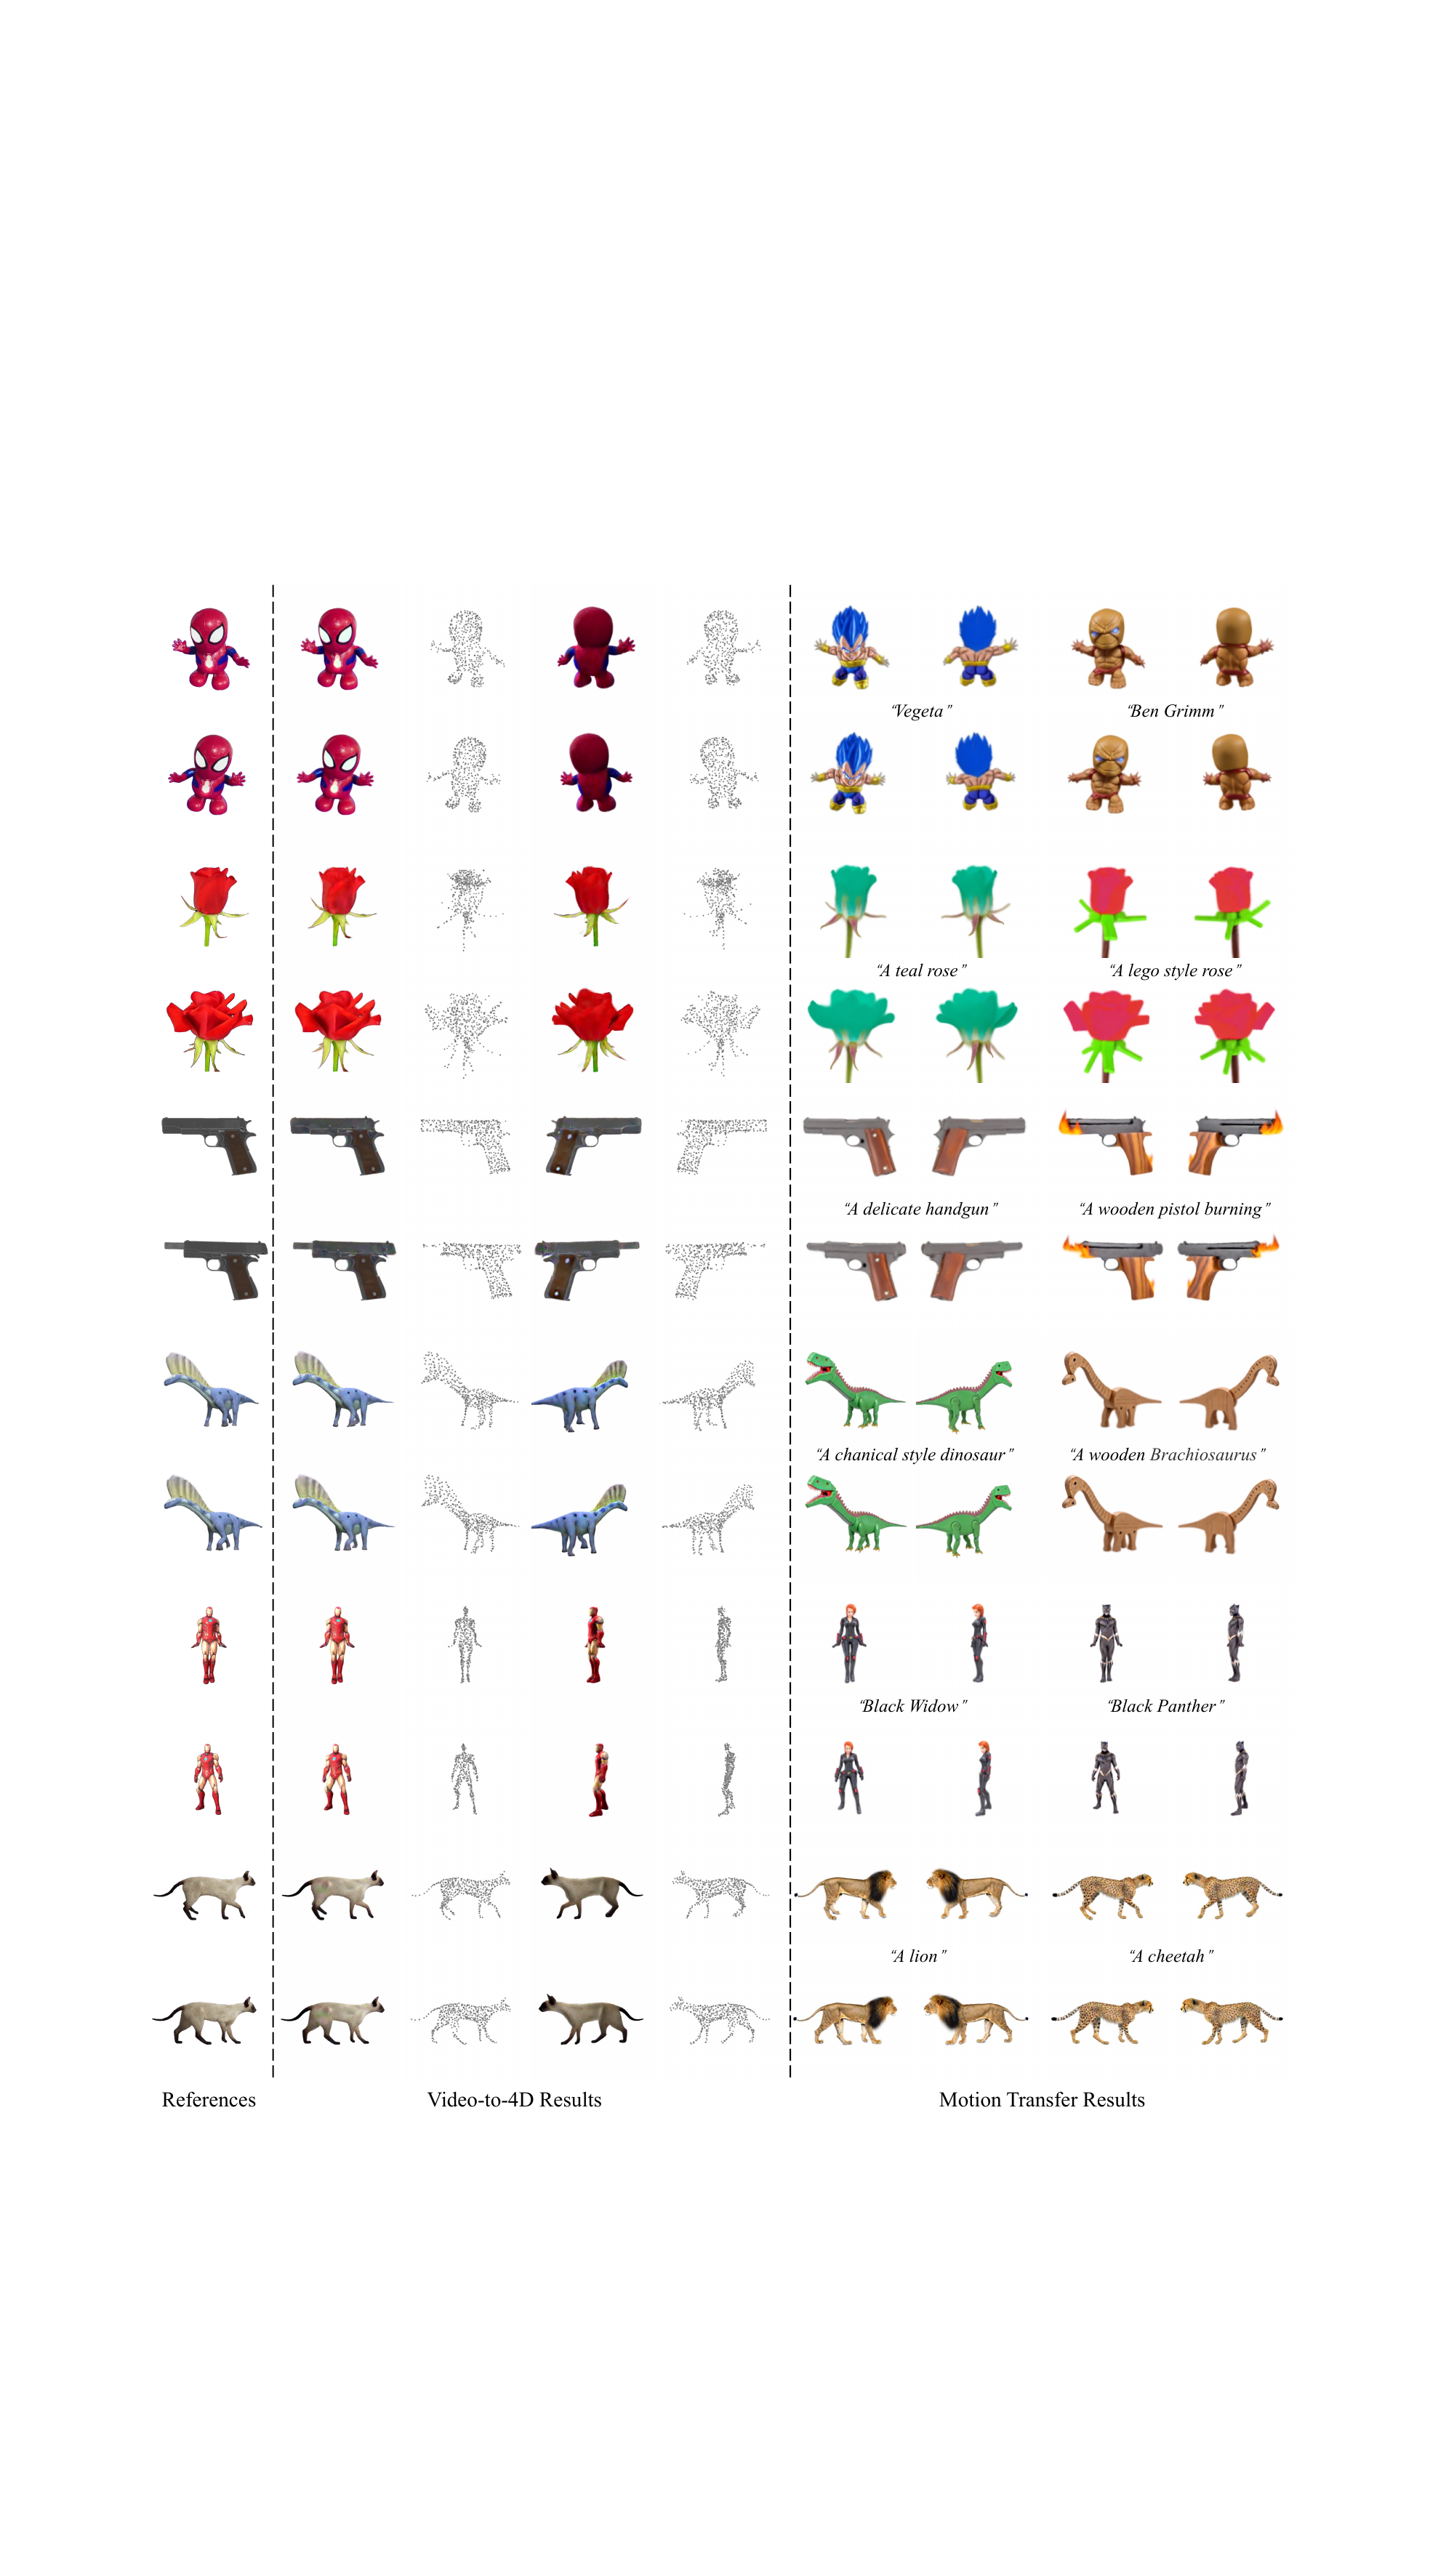}
\end{center}
\vspace{-.2in}
\caption{Additional application examples. (Best viewed when zoomed in.)}
\label{fig:supp_app}
\end{figure}
